# Supplementary material for: Copula variational inference
Source: arXiv:1506.03159 source file (2015-10-31)
Supplement: Supplementary file 1 [file sec_appendix.tex]

\section{Sampling from the copula-augmented variational distribution}
\label{sec:sampling}
We sample from the copula-augmented distribution by repeatedly doing inverse
transform sampling~\citep{devroye1986non}, also known as inverse CDF, on the
individual pair copulas and finally the marginals.
%This can be computed
%efficiently in worst-case complexity of $\mathcal{O}(md^2)$, where $m$ is the
%number of desired samples and $d$ is the dimension of the
%distribution.
More specifically, the sampling procedure is as follows:
\begin{enumerate}
\item Generate $\mbu=(\mbu_1,\ldots,\mbu_d)$ where each $\mbu_i\sim\mathcal{U}(0, 1)$.
\item Calculate $\mbv=(\mbv_1,\ldots,\mbv_d)$ which follows a joint uniform distribution with
dependencies given by the copula:
\begin{align*}
\mbv_1 &= \mbu_1\\
\mbv_2 &= Q_{2\g 1}^{-1}(\mbu_2\g \mbv_1)\\
\mbv_3 &= Q_{3\g 12}^{-1}(\mbu_3\g \mbv_1, \mbv_2)\\
&\setbox0\hbox{=}\mathrel{\makebox[\wd0]{\hfil\vdots\hfil}}\nonumber\\
\mbv_d &= Q_{d\g 12\cdots d-1}^{-1}(\mbu_d\g \mbv_1,\mbv_2,\ldots,\mbv_{d-1})
\end{align*}
Explicit calculations of the inverse of the conditional CDFs $Q^{-1}_{i|12\cdots
i-1}$ can be found in \citet{kurowicka2007sampling}. The
procedure loops through the $d(d-1)/2$ pair copulas and thus has worst-case
complexity of $\mathcal{O}(d^2)$.
\item Calculate $\mbz=(Q_1^{-1}(\mbv_1),\ldots,Q_d^{-1}(\mbv_d))$, which is a sample from
the copula-augmented distribution $q(\mbz; \mblambda,\mbeta)$.
\end{enumerate}
Evaluating gradients with respect to $\mblambda$ and $\mbeta$ easily follows from backpropagation, i.e., by applying the chain rule on this sequence of deterministic transformations.

\section{Choosing the tree structure and pair copula families}

We assume that the vine structure and pair copula families are
specified in order to perform \glsreset{CVI}\gls{CVI}, in the same way
one must specify the mean-field family for black box variational
inference \citep{ranganath2014black}. In general however, given a
factorization of the variational distribution, one can determine the
tree structure and pair copula families based on synthetic data of the
latent variables $z$.

During tree selection, enumerating and calculating all possibilities is
computationally intractable, as the number of possible vines on $d$ variables
grows factorially: there exist $d!/2\cdot 2^{{d-2\choose 2}}$ many choices
\citep{morales2010about}.  The most common approach in practice is to
sequentially select the maximum spanning tree starting from the initial tree
$T_1$, where the weights of an edge are assigned by absolute values of the
Kendall's $\tau$ correlation on each pair of random variables. Intuitively, the
tree structures are selected as to model the strongest pairwise dependencies.
This procedure of sequential tree selection follows
\citet{dissmann2012selecting}.

\if0
% Learning tree and families on subset of the data
sequential tree selection \citep{dissmann2012selecting} and Bayesian model
selection, based on maximizing the marginal likelihood, are run on a subset of
the data. We then fix them upon future iterations, requiring that one only
re-updates the copula parameters. In preliminary experiments we've found that
the tree structure and copula families do not change significantly upon future
iterations. As the procedure outlined in Algorithm \ref{alg:cvi-i} is very
flexible, one could reselect the vine's trees and copula families after a
certain number of iterations in order to further reduce the bias.
\fi

In order to select a family of distributions for each conditional bivariate
copula in the vine, one may employ Bayesian model selection, i.e., choose among
a set of families which maximizes the marginal likelihood. We note that both
the sequential tree selection and model selection are implemented in the
\texttt{VineCopula} package in R \citep{schepsmeier2015vine}, which makes it easy
for users to learn the structure and families for the copula-augmented
variational distribution.

We also list below the 16 bivariate copula families used in our experiments.

\begin{figure}[!h]
\begin{minipage}{\textwidth}
  \begin{minipage}[b]{0.49\textwidth}
    \centering
  \begin{tabular}{|l|l|l|}
  \hline
  \textbf{Family} & \textbf{Parameter} &  $\theta(\tau)$\\
  \hline
  Independent & --- & --- \\ \hline
  Gaussian               & $\theta \in [-1,1]$       &
  \multirow{2}{*}{$\sin\left(\dfrac{\pi}{2} \tau\right)$} \\\cline{1-2}
  Student-$t$            & $\theta \in [-1,1]$       & \\ \hline
  Clayton                & $\theta \in (0, \infty) $ & $2\tau/(1-\tau)$ \\ \hline
  Gumbel                 & $\theta \in [1,\infty)$   & $1/(1-\tau)$ \\ \hline
  Frank                  & $\theta \in (0, \infty)$  & \multirow{2}{*}{No closed form} \\\cline{1-2}
  Joe                    & $\theta \in (1, \infty)$  &\\\hline
  \end{tabular}
      \captionof{table}{\label{table:thetatau}The 16 bivariate copula families,
      with their parameter domains and expressed in terms of Kendall's $\tau$
      correlations, that we consider in experiments. We include rotated
      versions ($90^\circ$, $180^\circ$, and $270^\circ$) of the Clayton,
      Gumbel, and Joe copulas.}
    \end{minipage}
  \hfill
  \begin{minipage}[b]{0.49\textwidth}
    \centering
    \includegraphics[width=1.1\textwidth]{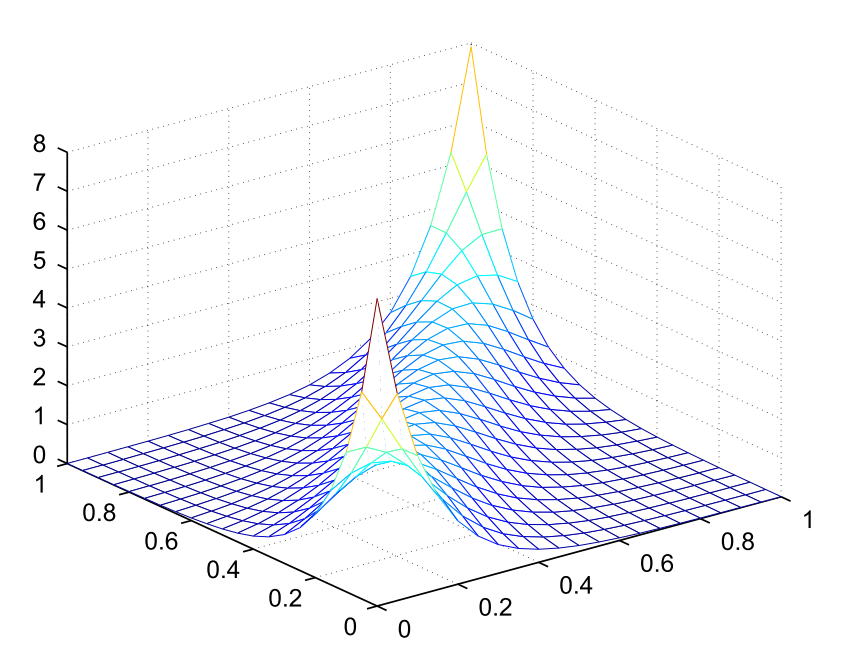}
    \captionof{figure}{Example of a Frank copula with correlation parameter 0.8,
    which is used to model weak symmetric tail dependencies.}
    % Taken from Kurowicka and Cooke (2007)
  \end{minipage}
\end{minipage}
\end{figure}

\section{Additional Gaussian mixture experiments}

We include figures showing the standard deviation estimates for $\mbmu$ and $\mbpi$ which were not included in the main paper. The results indicate the same pattern as for $\mbLambda$.

\begin{figure}[t]
  \centering
  \includegraphics[width=0.8\textwidth]{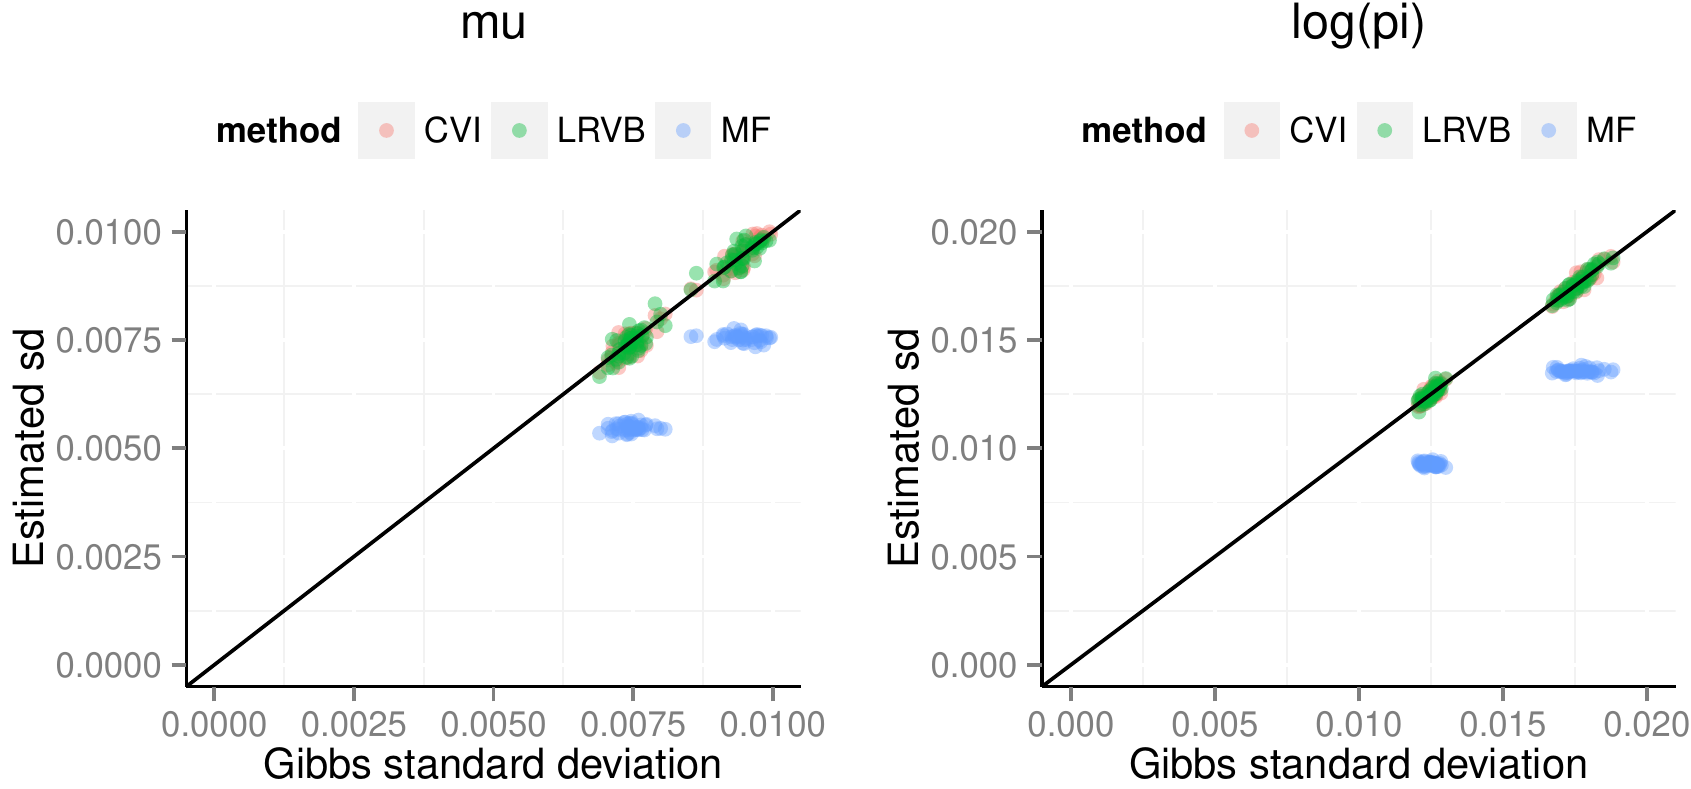}
  \caption{\label{fig:lrvb}Covariance estimates from
  copula variational inference (\gls{CVI}), mean-field (\gls{MF}), and
  linear response variational Bayes (\gls{LRVB}) to the ground truth
  (Gibbs samples). \gls{CVI} and \gls{LRVB} effectively capture dependence
  while \gls{MF} underestimates variance and forgets covariances.}
\end{figure}
